# Supplementary material for: Just Rotate it: Deploying Backdoor Attacks via Rotation Transformation
Source: arXiv:2207.10825 source file (2022-07-22)
Supplement: Supplementary file 1 [file appendix_cifar10.tex]

\newpage

\section{CIFAR10}

CIFAR10 is a relatively small dataset with 10 objects and 60,000 images in total. In poisoning data processing, we first rotate the selected images to the backdoored angle and center crop the image in order to keep all useful information. For example, if the backdoored angle is $45^{\circ}$, after rotating, we utilize the middle square from $\frac{2-\sqrt{2}}{4}$ to $\frac{2+\sqrt{2}}{4}$. As we mentioned before, to compare the benign baseline fairly, the clean images are also clipped to the same size. All images will then be resize back to 32 $\times$ 32 pixels. We use ResNet34 as the backbone of the victim model, which achieved more than 90 \% of clean accuracy of full size images. 

We begin by using the $5 \%$ of poisoning rate of backdoored images. Specifically, we utilize four different types of data augmentation in the training process, which are 1) No rotation augmentation, 2) $[-15^\circ, 15^\circ]$ rotation augmentation, 3) $[-30^\circ, 30^\circ]$ rotation augmentation, and 4) $[-45^\circ, 45^\circ]$ rotation augmentation. 

For implementation, we adopt \textbf{RandomRotation} function from the Pytorch library, where every image is rotated for an angle uniformly chosen from the given range. In fact, as we observed, a lot of previous literature did not even use rotation augmentation when implementing neural network. We also select the $[15^\circ, 30^\circ, 45^\circ]$ as the backdoored trigger to evaluate the performance. 

\begin{table}[H]
\begin{tabular}{@{}llccc@{}}
\toprule
\multicolumn{1}{l}{}     & No Rot. & $\pm 15^\circ$ Rot. & $\pm 30^\circ$ Rot. & $\pm 45^\circ$ Rot. \\ \midrule
\multicolumn{1}{c|}{RB: $15^\circ$} & \begin{tabular}[c]{@{}l@{}}97.04 \%\\ (-2.65\%)\end{tabular}                      & \begin{tabular}[c]{@{}c@{}}70.42 \%\\ (-0.59\%)\end{tabular}      & \begin{tabular}[c]{@{}c@{}}49.00 \%\\ (-3.21\%)\end{tabular}      & \begin{tabular}[c]{@{}c@{}}39.00 \%\\ (-3.43\%)\end{tabular}      \\ \midrule
\multicolumn{1}{c|}{RB: $30^\circ$} & \begin{tabular}[c]{@{}l@{}}99.14 \%\\ (-2.70\%)\end{tabular}                      & \begin{tabular}[c]{@{}c@{}}92.73 \%\\ (-2.09\%)\end{tabular}      & \begin{tabular}[c]{@{}c@{}}75.62 \%\\ (-1.31\%)\end{tabular}      & \begin{tabular}[c]{@{}c@{}}45.07 \%\\ (-3.41\%)\end{tabular}      \\ \midrule
\multicolumn{1}{l|}{RB: $45^\circ$} & \multicolumn{1}{c}{\begin{tabular}[c]{@{}c@{}}98.64 \%\\ (-10.08\%)\end{tabular}} & \begin{tabular}[c]{@{}c@{}}85.48 \%\\ (-2.03\%)\end{tabular}      & \begin{tabular}[c]{@{}c@{}}74.07 \%\\ (-2.40\%)\end{tabular}      & \begin{tabular}[c]{@{}c@{}}57.97 \%\\ (-3.02\%)\end{tabular}    \\ \bottomrule
\end{tabular}
\caption{ Evaluation of rotation trigger with 5\% poisoning rate in CIFAR10 dataset. The upper value stands for the success attack rate, followed by the standard accuracy degradation}
\label{table:0.05}
\end{table}

It can be seen from Table \ref{table:0.05} that our attacking performance is  effective overall. Even under the $\pm 45^\circ$ rotation augmentation, we can achieve nearly 0.6 attack success rate with negligible $(< 3.02\%)$ standard accuracy degradation. We also observe that larger rotation angle is more effective under most data augmentation settings. For example, compared with  $15^\circ$, $45^\circ$ can boost the attacking performance for about 19\% in last column.  Moreover, we find that data augmentation is an effective method to mitigate our rotation backdoor strategy by comparing the different augmentation strength. In general, the standard accuracy degradation is less than 4 \% except for the $45^\circ$ trigger with no rotation augmentation.

Next, we evaluate the performance with various extents of injection rate by using the $45^\circ$ as the backdoored trigger. In Table \ref{table:CIFAR45}, as we expect, larger injection rate can generate more effective attacks. Also, we point out that if no rotation augmentation is used, 1 \% of poisoning samples can lead to over 90 \% of attack success rate. Therefore, as a host of implementations of neural network do not use rotation as augmentation, 

In addition, we observe that applying rotation backdoor attacks for the model with no rotation augmentation is likely to have large standard accuracy degradation.

\begin{table}[H]
\begin{tabular}{@{}lcccc@{}}
\toprule
\multicolumn{1}{l}{}     & No Rot. & \pm 15^\circ Rot. & \pm 30^\circ Rot. & \pm 45^\circ Rot. \\ \midrule
\multicolumn{1}{c|}{Inj. Rate: 1\%}  & \begin{tabular}[c]{@{}c@{}}93.56\%\\ (-8.19\%)\end{tabular}  & \begin{tabular}[c]{@{}c@{}}46.85\%\\ (-2.62\%)\end{tabular}       & \begin{tabular}[c]{@{}c@{}}29.84\%\\ (-1.05\%)\end{tabular}       & \begin{tabular}[c]{@{}c@{}}15.28\%\\ (-0.45\%)\end{tabular}       \\ \midrule
\multicolumn{1}{c|}{Inj. Rate: 5\%}  & \begin{tabular}[c]{@{}c@{}}98.64\%\\ (-10.08\%)\end{tabular} & \begin{tabular}[c]{@{}c@{}}85.48\%\\ (-2.03\%)\end{tabular}       & \begin{tabular}[c]{@{}c@{}}74.07\%\\ (-2.40\%)\end{tabular}       & \begin{tabular}[c]{@{}c@{}}57.97\%\\ (-3.02\%)\end{tabular}       \\ \midrule
\multicolumn{1}{l|}{Inj. Rate: 10\%} & \begin{tabular}[c]{@{}c@{}}99.66\%\\ (-8.87\%)\end{tabular}  & \begin{tabular}[c]{@{}c@{}}98.25\%\\ (-3.32\%)\end{tabular}       & \begin{tabular}[c]{@{}c@{}}88.05\%\\ (-3.80\%)\end{tabular}       & \begin{tabular}[c]{@{}c@{}}76.03\%\\ (-2.92\%)\end{tabular}       \\ \bottomrule
\end{tabular}
\caption{ Evaluation of $45^{\circ}$ rotation trigger in CIFAR10 dataset under different injection rate. The upper value stands for the success attack rate, followed by the standard accuracy degradation}
\label{table:CIFAR45}
\end{table}

Lastly, we present all additional results we obtained.  Again, we select $[15^\circ, 30^\circ, 45^\circ]$ as the backdoored trigger and 4 data augmentation methods to evaluate the performance under 1\% and 10\% injection rate.  

\begin{table}[H]
\begin{tabular}{@{}llccc@{}}
\toprule
\multicolumn{1}{l}{}     & No Rot. & $\pm 15^\circ$ Rot. & $\pm 30^\circ$ Rot. & $\pm 45^\circ$ Rot. \\ \midrule
\multicolumn{1}{c|}{RB: $15^\circ$} & \begin{tabular}[c]{@{}l@{}}30.63 \%\\ (+0.11\%)\end{tabular}                      & \begin{tabular}[c]{@{}c@{}}16.3 \%\\ (-0.91\%)\end{tabular}      & \begin{tabular}[c]{@{}c@{}}8.4 \%\\ (-0.81\%)\end{tabular}      & \begin{tabular}[c]{@{}c@{}}9.75 \%\\ (-1.35\%)\end{tabular}      \\ \midrule
\multicolumn{1}{c|}{RB: $30^\circ$} & \begin{tabular}[c]{@{}l@{}}64.34 \%\\ (-1.72\%)\end{tabular}                      & \begin{tabular}[c]{@{}c@{}}36.62 \%\\ (-1.49\%)\end{tabular}      & \begin{tabular}[c]{@{}c@{}}14.3 \%\\ (-1.31\%)\end{tabular}      & \begin{tabular}[c]{@{}c@{}}11.18 \%\\ (-0.89\%)\end{tabular}      \\ \midrule
\multicolumn{1}{l|}{RB: $45^\circ$} & \begin{tabular}[c]{@{}c@{}}93.56\%\\ (-8.19\%)\end{tabular}  & \begin{tabular}[c]{@{}c@{}}46.85\%\\ (-2.62\%)\end{tabular}       & \begin{tabular}[c]{@{}c@{}}29.84\%\\ (-1.05\%)\end{tabular}   
 &  \begin{tabular}[c]{@{}c@{}}15.28\%\\ (-0.45\%)\end{tabular}     \\ \bottomrule
\end{tabular}
\caption{ Additional Evaluation of rotation trigger with 1\% poisoning rate in CIFAR10 dataset.}
\label{table:0.01}
\end{table}

\begin{table}[H]
\begin{tabular}{@{}llccc@{}}
\toprule
\multicolumn{1}{l}{}     & No Rot. & $\pm 15^\circ$ Rot. & $\pm 30^\circ$ Rot. & $\pm 45^\circ$ Rot. \\ \midrule
\multicolumn{1}{c|}{RB: $15^\circ$} & \begin{tabular}[c]{@{}l@{}}99.32 \%\\ (-3.74\%)\end{tabular}                      & \begin{tabular}[c]{@{}c@{}}87.06 \%\\ (-2.22\%)\end{tabular}      & \begin{tabular}[c]{@{}c@{}}84.57 \%\\ (-3.21\%)\end{tabular}      & \begin{tabular}[c]{@{}c@{}}72.18 \%\\ (-5.13\%)\end{tabular}      \\ \midrule
\multicolumn{1}{c|}{RB: $30^\circ$} & \begin{tabular}[c]{@{}l@{}}99.71 \%\\ (-6.67\%)\end{tabular}                      & \begin{tabular}[c]{@{}c@{}}99.02 \%\\ (-3.26\%)\end{tabular}      & \begin{tabular}[c]{@{}c@{}}86.94 \%\\ (-8.02\%)\end{tabular}      & \begin{tabular}[c]{@{}c@{}}73.87 \%\\ (-3.45\%)\end{tabular}      \\ \midrule
\multicolumn{1}{l|}{RB: $45^\circ$} & \begin{tabular}[c]{@{}c@{}}99.66\%\\ (-8.87\%)\end{tabular}  & \begin{tabular}[c]{@{}c@{}}98.25\%\\ (-3.32\%)\end{tabular}       & \begin{tabular}[c]{@{}c@{}}88.05\%\\ (-3.80\%)\end{tabular}       & \begin{tabular}[c]{@{}c@{}}76.03\%\\ (-2.92\%)\end{tabular}       \\ \bottomrule
\end{tabular}
\caption{ Additional Evaluation of rotation trigger with 10\% poisoning rate in CIFAR10 dataset.}
\label{table:0.1}
\end{table}

\begin{figure}[h!]
\begin{center}
\includegraphics[width=0.47\textwidth]{Fig/analysis_ResNet34BRT901005.pdf}
\caption{ Visually Interpretation of rotation backdoored model on CIFAR10 with $90 ^\circ$ as backdoored angle without rotation augmentation. }
\label{fig:analysis_ResNet34BRT901005}
\end{center}
\end{figure}

\begin{figure}[h!]
\begin{center}
\includegraphics[width=0.47\textwidth]{Fig/analysis_ResNet34BRT902005.pdf}
\caption{ Visually Interpretation of rotation backdoored model on CIFAR10 with $90 ^\circ$ as backdoored angle with $\pm 15^\circ$ Rotation augmentation}
\label{fig:analysis_ResNet34BRT902005}
\end{center}
\end{figure}

% \begin{figure}[h!]
% \begin{center}
% \includegraphics[width=0.47\textwidth]{Fig/analysis_ResNet34BRT903005.pdf}
% \caption{ Visually Interpretation of rotation backdoored model on CIFAR10 with $90 ^\circ$ as backdoored angle with $\pm 30^\circ$ Rotation augmentation}
% \label{fig:analysis_ResNet34BRT903005}
% \end{center}
% \end{figure}

% \begin{figure}[h!]
% \begin{center}
% \includegraphics[width=0.47\textwidth]{Fig/analysis_ResNet34BRT904005.pdf}
% \caption{ Visually Interpretation of rotation backdoored model on CIFAR10 with $90 ^\circ$ as backdoored angle with $\pm 45^\circ$ Rotation augmentation }
% \label{fig:analysis_ResNet34BRT904005}
% \end{center}
% \end{figure}
